# Supplementary material for: Unleashing the Power of LLM to Infer State Machine from the Protocol Implementation
Source: arXiv:2405.00393 source file (2025-03-27)
Supplement: Supplementary file 1 [file Appendix.tex]

%%
%% If your work has an appendix, this is the place to put it.
\appendix

\section{Research Methods}

\subsection{Part One}

\subsection{Part Two}

\section{Online Resources}
